# Supplementary material for: Learning a Distributed Hierarchical Locomotion Controller for Embodied Cooperation
Source: arXiv:2407.06499 source file (2024-10-26)
Supplement: Supplementary file 1 [file appendix2.tex]

\section{Supplementary Appendix}
\label{sec:appendix2}
\subsection{Comparison to Other MARL Alogithms }
We supplement comparison between the proposed distributed HRL method to other state-of-the-art MARL approaches based on the article BenchMARL: Benchmarking Multi-Agent Reinforcement Learning Algorithms. Specifically, we compare our method with MAPPO and MASAC since the Isaac Sim algorithm is nested within the RLGame and the CTDE algorithms supported by RLGame are only MAPPO and MASAC. The picture on the left below shows the results. We find that MAPPO converges a little faster than distributed method because it is centrally trained with global observations. However, the CTDE algorithm has worse performance and take much more training time when facing a larger number of agents, which will be demonstrated in our experiments in the next section.
 
 \begin{figure}[h]
  \centering
  % First image
  \begin{minipage}{0.33\textwidth}
    \centering
    \includegraphics[width=\linewidth]{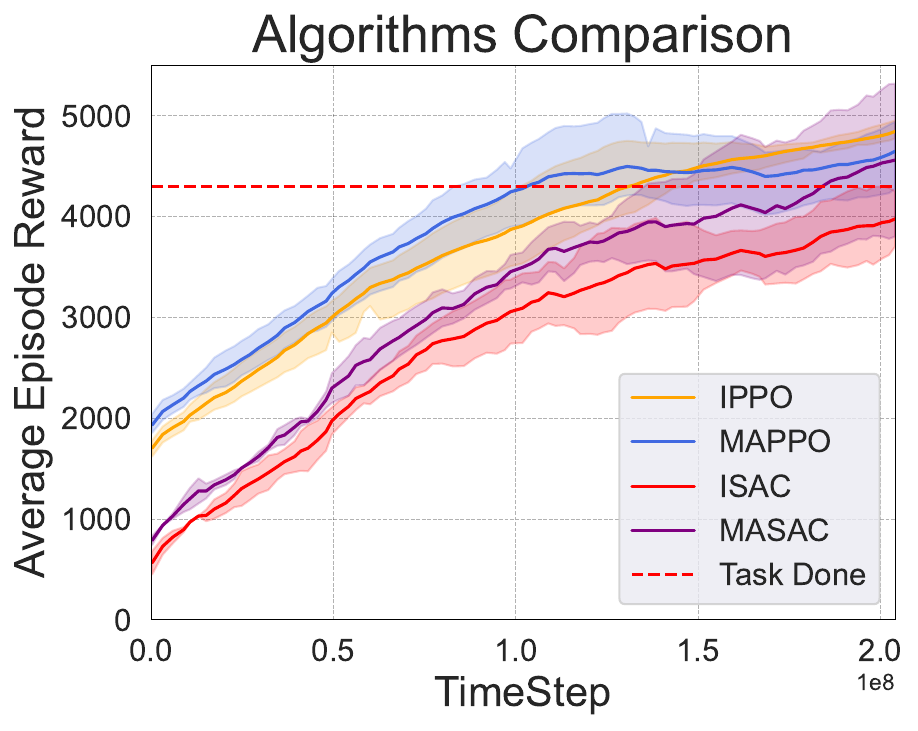} % Adjust your image file name
  \end{minipage}%
  % Second image
  \begin{minipage}{0.33\textwidth}
    \centering
    \includegraphics[width=\linewidth]{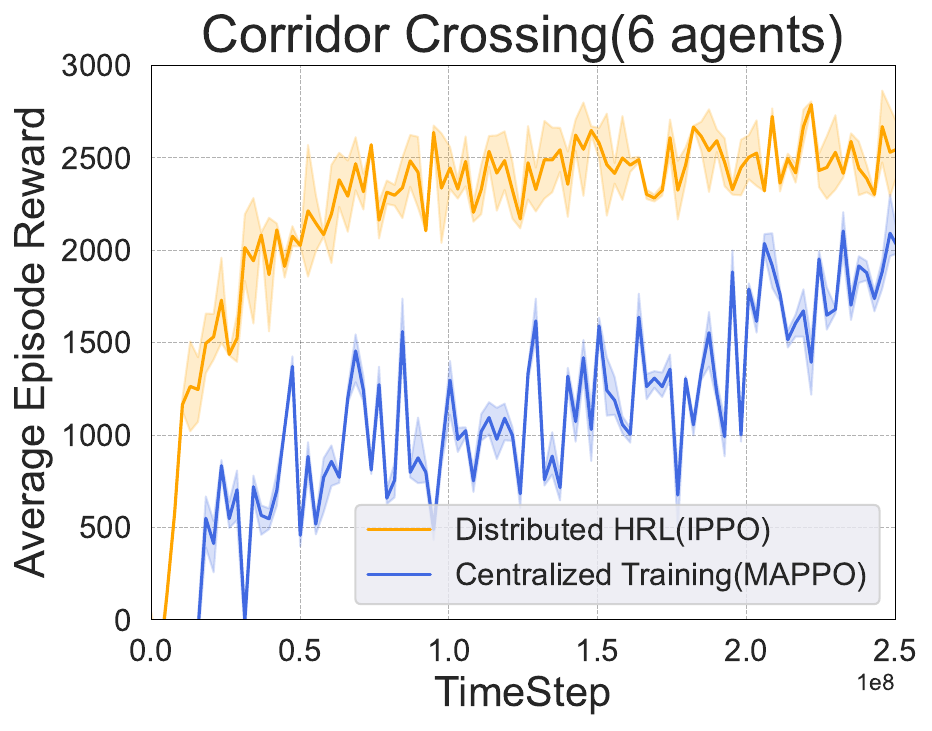} % Adjust your image file name
  \end{minipage}%
  % Third image
  \begin{minipage}{0.33\textwidth}
    \centering
    \includegraphics[width=\linewidth]{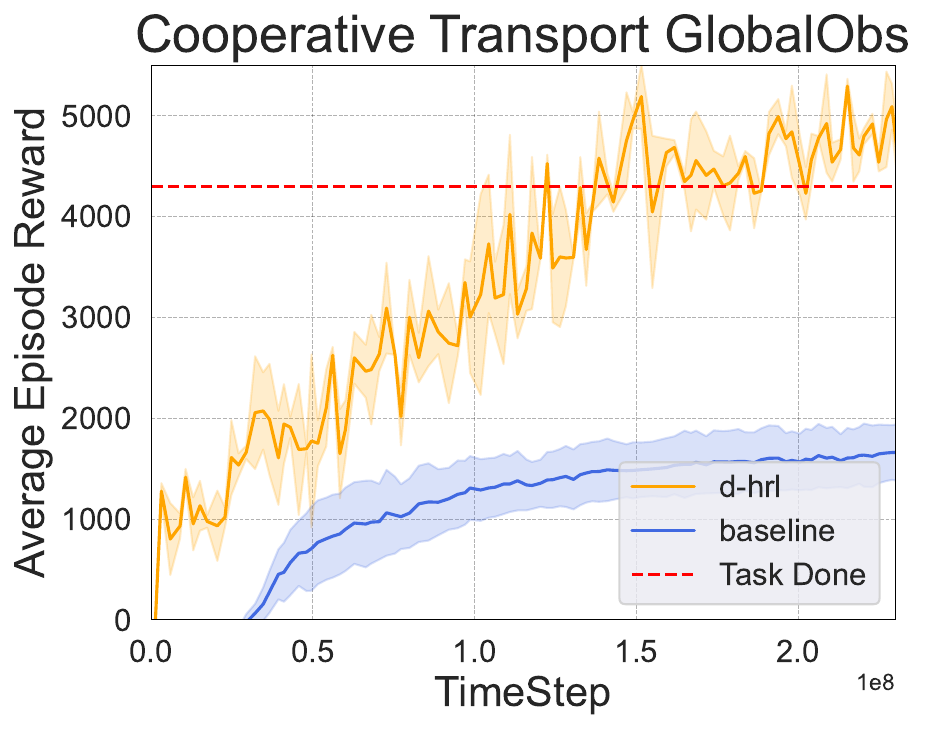} % Adjust your image file name
  \end{minipage}
 % You can add a descriptive caption for the entire figure.
  \label{fig:cross_typical_result} % This label can be used for referencing the entire figure.
\end{figure}

\subsection{A Larger Agent's Number Experiment}
 We supplement the experiment to show the advantages of our fully decentralized method over the CTDE method when the number of agents increases. The most appropriate task to show is Corridor Crossing because as the number of agents increases, the difficulty of the task Cooperative Transport decreases, while Ravine Bridging is too complex and the completion rate is too low when the number of agents is large. So we add the number of agents to 6 in corridor crossing. And the picture in the middle above shows the result, the reward of centralized training grows slow and ultimately not converge.

\subsection{Cooperative Transport With Global Observation}
 We still want to emphasize the decisive role of spatiotemporal memory in long-horizon team collaboration tasks. However, it is true that we did not take the influence of spatiotemporal memory to the partial observation into consideration. So we conduct an additional ablation experiment to verify whether spatiotemporal memory is still decisive when its influence on partial observation is excluded. We choose the typical task Cooperative Transport to show. Now we give all the absolute position of other agents and cylinder to each agents to exclude the influence on partial observation. We still find that the baseline algorithm without spatiotemporal memory could only get really low rewards and fail to learning cooperation strategy. In this case, We believe that our analysis about effectiveness of spatiotemporal memory is still reasonable. 

\subsection{Limitation}
Despite the encouraging findings, it is imperative to acknowledge the limitation of our research. Firstly, although the hierarchical network method enables our framework with some ability to solve long-horizon problems, its ability to solve complex problems is still limited since all layers still fully trained base reinforcement learning. And it still has difficulty to work in many more complex tasks.
Moreover, during the training of the three tasks we presented, we were also limited by the fact that reinforcement learning algorithms are entirely based on random exploration. So we mainly relied on continuous reward shaping and increasing the total training steps to achieve better training results. We believe that if we want to solve more complex tasks with more intelligent agents participating, it may not be enough to rely solely on our network, and additional planning-based guidance may be needed at the upper level. 
Finally, our work is indeed more algorithmic and simulation benchmark-oriented, and we have not explored robots with more complex morphology. Despite we have already demonstrated the promising results of our method on some tasks and witnessed the emergence of cooperative behavior.There is still a considerable engineering workloads required in terms of controlling and transferring.

\subsection{Training pipeline of Ravine Bridging}
As we mentioned in Appendix A.2, the Ravine Bridging task is more intricate, which means we have to provide more guidance. And the agent's behavior is divided into stages, so the training process must also be divided accordingly. Therefore, there is a series of pre-train courses to complete this task. For the agent in the ravine, its upper layer receives observations that include the position of the bridging stone, its own position, and the position of the Ant on the plane closest to the ravine. The Ant on the plane receives observations that includes the position of the stone, its own position, and the x coordinate of the ravine and the finish line. Before training together, we train them separately first to obtain their featured skills. For the agents in the ravine, we randomize the position of the Ant closest to the ravine in the input and give the agent a y-axis direction distance reward of the distance between the stone and the randomize Ant's position, so that the agent in the ravine has the ability to move the stone to the closest Ant on the plane. For the agents on the plane, we add a reward for the x-axis direction distance to the finish line and a punishment for falling (death), so that it learns the ability to move straight towards the finish line and stop before falling into the ravine. Finally, we train all of them together, and once an Ant crosses the finish line, we give all of them a large sparse reward. For all the reward precise equations mentioned above, we will list them in the following section.

\subsection{Reward Details}
\subsubsection{Lower layer}
\subsubsubsection{Target paradigm}

\begin{tabular}{|>{\raggedright}m{5cm}|m{10cm}|}
    \hline
    \textbf{Reward Type} & \textbf{Formula} \\ \hline
    Distance to target reward & \(5 \times \left(\frac{1}{1 + \sqrt{(\text{agent\_pos}[:,0] - \text{target\_pos}[:,0])^2 + (\text{agent\_pos}[:,1] - \text{target\_pos}[:,1])^2}}\right)\) \\ \hline
    Alive reward & 0.5 \\ \hline
    Up reward & 0.1 \\ \hline
    Action cost & \(0.005 \times \text{action cost}\) \\ \hline
    Energy cost & \(0.05 \times \text{energy cost}\) \\ \hline
    Dof at limit cost & \(0.1 \times \text{dof at limit cost}\) \\ \hline
\end{tabular}
  
\subsubsubsection{Velocity paradigm}

\begin{tabular}{|>{\raggedright}m{5cm}|m{10cm}|}
    \hline
    \textbf{Reward Type} & \textbf{Formula} \\ \hline
    Vel reward & \(5 \times \text{clamp}(\text{vel}[:,:2] \cdot \text{cmd\_direction}, \text{max} = 1)\) \\ \hline
    Alive reward & 0.5 \\ \hline
    Up reward & 0.1 \\ \hline
    Action cost & \(0.005 \times \text{action cost}\) \\ \hline
    Energy cost & \(0.05 \times \text{energy cost}\) \\ \hline
    Dof at limit cost & \(0.1 \times \text{dof at limit cost}\) \\ \hline
\end{tabular}

\subsubsection{Upper layer}
\subsubsubsection{Cooperative Transport}

\begin{tabular}{|>{\raggedright}m{6cm}|m{10cm}|}
    \hline
    \textbf{Reward Type} & \textbf{Formula} \\ \hline
    Cylinder-target distance reward & \(10 \times \left(\frac{1}{1 + \sqrt{(\text{cylinder\_pos}[:,0] - \text{target\_pos}[:,0])^2 + (\text{cylinder\_pos}[:,1] - \text{target\_pos}[:,1])^2}}\right)\) \\ \hline
    Agent-cylinder distance reward & \(5 \times \left(\frac{1}{1 + \sqrt{(\text{agent\_pos}[:,0] - \text{cylinder\_pos}[:,0])^2 + (\text{agent\_pos}[:,1] - \text{cylinder\_pos}[:,1])^2}}\right)\) \\ \hline
    Agent-target distance reward & \(5 \times \left(\frac{1}{1 + \sqrt{(\text{agent\_pos}[:,0] - \text{target\_pos}[:,0])^2 + (\text{agent\_pos}[:,1] - \text{target\_pos}[:,1])^2}}\right)\) \\ \hline
    Reach destination reward & 50 (all agents) \\ \hline
\end{tabular}

\subsubsubsection{Cross Corridor}

 \begin{tabular}{|>{\raggedright}m{6cm}|m{10cm}|}
    \hline
    \textbf{Reward Type} & \textbf{Formula} \\ \hline
    Reach destination reward & 50 (all agents) \\ \hline
    Agent-target distance reward & \(5 \times \left(\frac{1}{1 + \sqrt{(\text{agent\_pos}[:,0] - \text{target\_pos}[:,0])^2 + (\text{agent\_pos}[:,1] - \text{target\_pos}[:,1])^2}}\right)\) \\ \hline
\end{tabular}

\subsubsubsection{Ravine Bridging}

\begin{tabular}{|>{\raggedright}m{6cm}|m{10cm}|}
    \hline
    \textbf{Reward/Punishment Type} & \textbf{Formula} \\ \hline
    Ravine pretrain: Distance of stone and nearest agent reward & \(5 \times \left(\frac{1}{1 + |\text{stone\_y} - \text{agent\_y}|}\right)\) \\ \hline
    Plane pretrain: Distance to destination line reward & \(5 \times \left(\frac{1}{1 + |\text{destination\_x} - \text{agent\_x}|}\right)\) \\ \hline
    Plane pretrain: Falling down punishment & -20 \\ \hline
    Integrated training: Pass destination line reward & 50 (all agents) \\ \hline
\end{tabular}
